# Supplementary material for: Metastable Interlayer Frenkel Pair Defects by Dipole-like Strain Fields for Dimensional Distortion in Black Phosphorus
Source: arXiv:1912.00376 source file (2019-12-01)
Supplement: Supplementary file 1 [file Supplemental_Material.pdf]

## Supplemental Material

# Metastable Interlayer Frenkel Pair Defects by Dipole-like Strain Fields for Dimensional Distortion in Black Phosphorus

Devesh R. Kripalani,[1,2] Yongqing Cai,[3,*] Ming Xue,[2] and Kun Zhou[1,†]

[1]*School of Mechanical and Aerospace Engineering, Nanyang Technological University, Singapore 639798, Singapore*

[2]*Infineon Technologies Asia Pacific Pte Ltd, Singapore 349282, Singapore*

[3]*Joint Key Laboratory of the Ministry of Education, Institute of Applied Physics and Materials Engineering, University of Macau, Taipa, Macau, China*

[*] yongqingcai@um.edu.mo

[†] kzhou@ntu.edu.sg

## I. STACKING REGISTRY OF BILAYER PHOSPHORENE

Bilayer phosphorene can adopt several possible stacking orders, giving rise to remarkably different structural, electronic and optical properties due to the presence of strong interlayer coupling.[1,2] In this work, we consider the relative structural stability of four distinct stacking orders, AA, AB, AC and AD, as shown in Fig. S1(a), where the top (purple) and bottom (green) layers are denoted as layers 1 and 2, respectively. AA-stacked phosphorene represents the reference configuration, in which both monolayers are in direct vertical alignment with one another (i.e. zero relative in-plane translation). With layer 1 fixed in its reference position, the AB (AD) stacking order can be described by a half-lattice translation of layer 2 in the zigzag (armchair) direction, while a superposition of these two translations form the basis of the AC stacking order.

The intralayer geometry of the bilayer is symmetric in the normal direction and can be characterized by its lattice constants ($a$, $b$), bond lengths ($r_1$, $r_1$', $r_2$), bond angles ($\theta_1$, $\theta_1$', $\theta_2$, $\theta_2$') and thickness $t$. The interlayer distance $d$ of the various stacking orders are optimized by pre-fitting DFT-calculated results to the universal binding energy relation (UBER),[3] as described by Eq. (S1). Here, $E_{\mathrm{BL}}$ and $E_{\mathrm{ML}}$ refer to the DFT-calculated total energies of the bilayer and monolayer repectively, while $A_0$ is the equilibrium in-plane area of the simulation cell. In accordance with UBER, the binding energy $E_{\mathrm{b}}$ is fundamentally dependent on three parameters - the equilibrium binding energy $E_0$, the equilibrium interlayer distance $d_0$ and the equilibrium elastic modulus of separation ${E_{\mathrm{b}}}''(d_0)$.

$$E_{\mathrm{b}}(d) = \frac{E_{\mathrm{BL}}(d) - 2E_{\mathrm{ML}}}{2A_0} = E_0(1+u)e^{-u}, \quad \text{where } u = (d-d_0)\left[\frac{{E_{\mathrm{b}}}''(d_0)}{-E_0}\right]^{\frac{1}{2}} \tag{S1}$$

The effect of interlayer distance on binding energy for the various stacking orders are shown in Fig. S1(b). The relaxed geometry, cohesive energy $E_{\mathrm{c}}$ and UBER-fitted parameters (before and after DFT optimization) of AA-, AB-, AC- and AD-stacked bilayer phosphorene are summarized in Table S1. Relevant data obtained for the monolayer are also included to provide a basis for comparison. The results calculated in this work show good agreement with that of other theoretical publications.[1,2,4] In general, we find small differences in lattice constants, bond lengths, bond angles and layer thickness between stacking orders, which lie within 0.7% of those in the monolayer. However, the interlayer distance varies significantly

with stacking order, from 3.197 Å in the AB-stacked bilayer to 3.769 Å in the AC-stacked configuration. The structural stability, from the most to least stable stacking order, follow AB > AD > AA > AC, in line with their relative cohesive energy, binding energy and elastic modulus of separation. Particularly, the most favourable AB-stacked bilayer exhibits the highest cohesive energy (3.517 eV/atom), most negative binding energy (-0.231 J/m$^2$) and highest elastic modulus of separation (3.756 GPA/Å). While the impact of DFT optimization on the UBER-fitted parameters is immaterial to the conclusion, numerical deviations do arise as a result of full structural relaxation during DFT calculations. Nevertheless, UBER demonstrates good applicability as a robust first-approximation for exploring the stacking attributes of van der Waals layered materials such as phosphorene (see Fig. S1(c)).

## II. THERMODYNAMIC STABILITY ANALYSIS

The room-temperature thermodynamic stability of the $B_2$ I-V pair is evaluated via *ab initio* molecular dynamics (AIMD) simulations using the optB88-vdW exchange-correlation functional. Finite temperature Γ-point calculations in the canonical (NVT) ensemble are performed at 300 K and for a period of 10 ps with a time step of 1 fs. The structural stability can be evaluated by the root-mean-square deviation (RMSD) and root-mean-square fluctuation (RMSF) of the system.[5,6] The RMSD of a group of $N$ atoms relative to a reference structure as a function of time $t$ is given by

$$\mathrm{RMSD}(t) = \sqrt{\frac{1}{N}\sum_{i=1}^{N}\left(r_i(t) - r_i^0\right)^2} \tag{S2}$$

where $r_i$ and $r_i^0$ refer to the instantaneous and reference ($t = 0$) position of atom $i$, respectively. The RMSF of each atom in the lattice is defined as the discrete time average

$$\mathrm{RMSF}_i = \sqrt{\frac{1}{T}\sum_{t=0}^{T}\left(r_i(t) - \langle r_i\rangle\right)^2} \tag{S3}$$

where $\langle r_i\rangle$ is the average position of atom $i$ over the simulation period $T$.

Our results from AIMD simulations are presented in Fig. S2. Stable temperature and RMSD cycling at 300 K indicate that the $B_2$ I-V pair can exhibit good structural stability

at room temperature. Furthermore, as shown in Fig. S2(c), the RMSF of phosphorus atoms is generally low across the lattice (below 0.4 Å), with relatively strong peaks corresponding to selected sites at the heart of the Frenkel defect.

---


[1] J. Dai and X. C. Zeng, J. Phys. Chem. Lett. **5**, 1289 (2014).

[2] T. Zhang, J.-H. Lin, Y.-M. Yu, X.-R. Chen, and W.-M. Liu, Sci. Rep. **5**, 13927 (2015).

[3] J. H. Rose, J. R. Smith, and J. Ferrante, Phys. Rev. B **28**, 1835 (1983).

[4] V. Wang, Y. Kawazoe, and W. T. Geng, Phys. Rev. B **91**, 045433 (2015).

[5] D. L. Theobald, Acta Cryst. **A61**, 478 (2005).

[6] B. P. Welford, Technometrics **4**, 419 (1962).

[7] J. P. Perdew, K. Burke, and M. Ernzerhof, Phys. Rev. Lett. **77**, 3865 (1996).

[8] J. Heyd, G. E. Scuseria, and M. Ernzerhof, J. Chem. Phys. **118**, 8207 (2003).

[9] J. Heyd, G. E. Scuseria, and M. Ernzerhof, J. Chem. Phys. **124**, 219906 (2006).

[10] Y. Cai, G. Zhang, and Y.-W. Zhang, Sci. Rep. **4**, 6677 (2014).

[11] J. Qiao, X. Kong, Z.-X. Hu, F. Yang, and W. Ji, Nat. Commun. **5**, 4475 (2014).

[12] H. Liu, A. T. Neal, Z. Zhu, Z. Luo, X. Xu, D. Tománek, and P. D. Ye, ACS Nano **8**, 4033 (2014).

[13] R. W. Keyes, Phys. Rev. **92**, 580 (1953).

[14] D. Warschauer, J. Appl. Phys. **34**, 1853 (1963).

[15] Y. Maruyama, S. Suzuki, K. Kobayashi, and S. Tanuma, Physica B+C **105**, 99 (1981).

[16] S. Narita, Y. Akahama, Y. Tsukiyama, K. Muro, S. Mori, S. Endo, M. Taniguchi, M. Seki, S. Suga, A. Mikuni, *et al.*, Physica B+C **117**, 422 (1983).

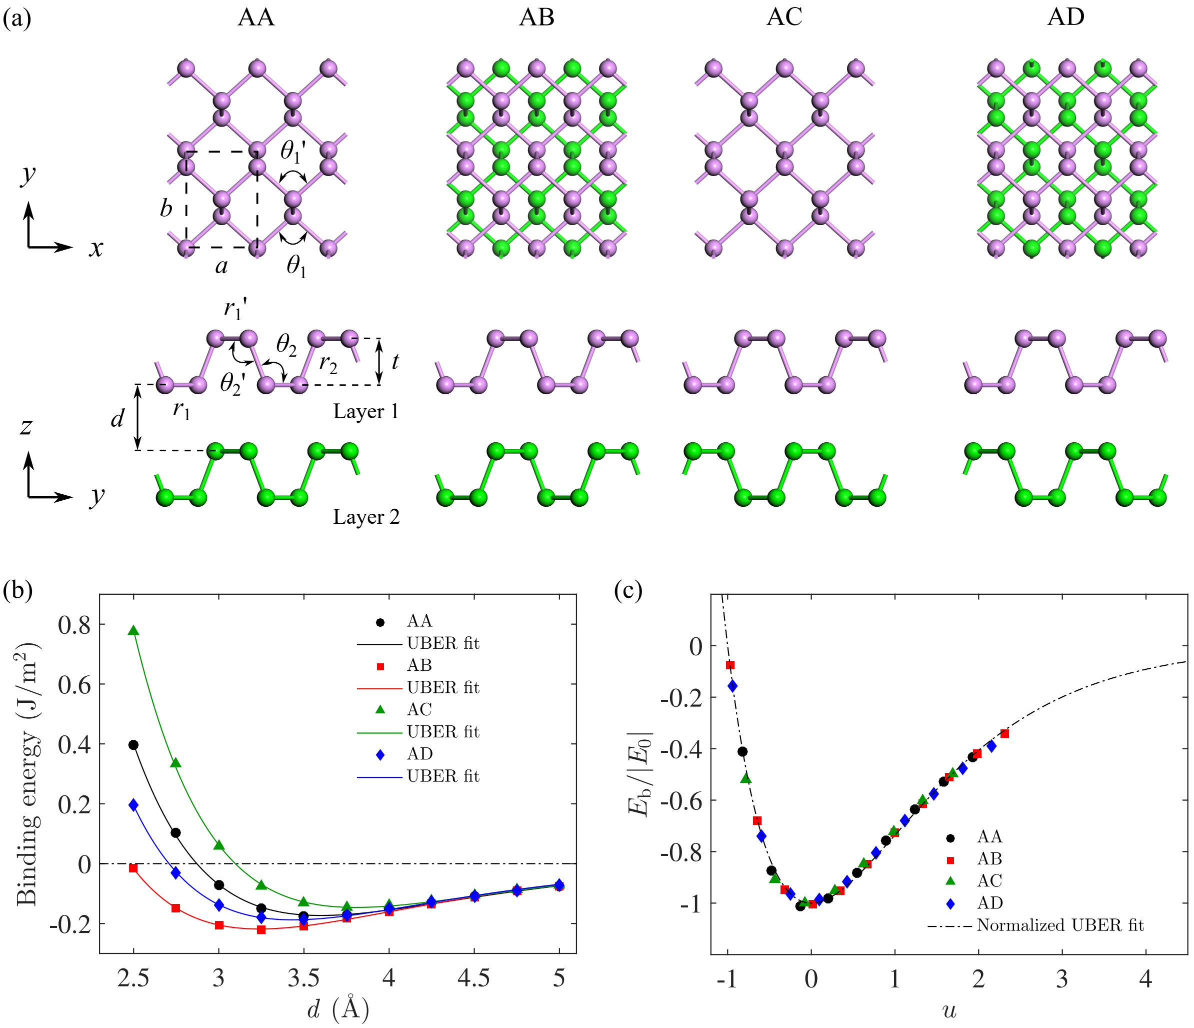


FIG. S1. (a) The structural configurations of AA-, AB-, AC- and AD-stacked bilayer phosphorene (top and side views). (b) The variation of binding energy with interlayer distance for AA- (black), AB- (red), AC- (green) and AD-stacked (blue) bilayer phosphorene. The data points are calculated from density functional theory (DFT) and fitted to the universal binding energy relation (UBER). (c) Normalized results of (b) expressed in the general form of UBER.

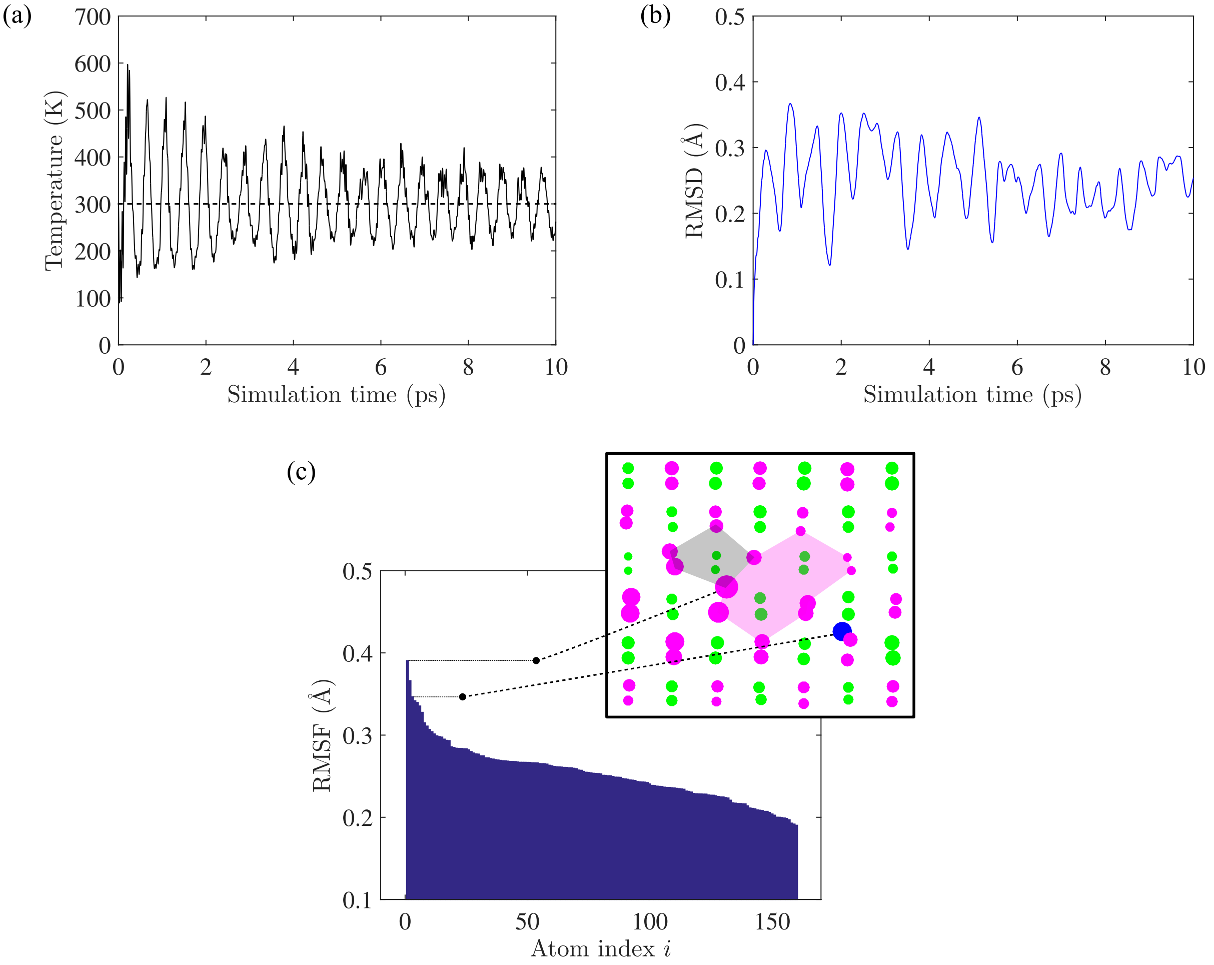


FIG. S2. *Ab initio* molecular dynamics simulation results at 300 K, showing the oscillations in (a) temperature, and (b) RMSD of the $B_2$ I-V pair over 10 ps. (c) RMSF distribution of phosphorus atoms across the lattice ($i$ = 1, 2, ..., 160). The inset denotes the average positions of atoms surrounding the defect (top view) in layer 1 (purple), layer 2 (green) and at the interstitial site (blue) with markers scaled according to their respective RMSF values.

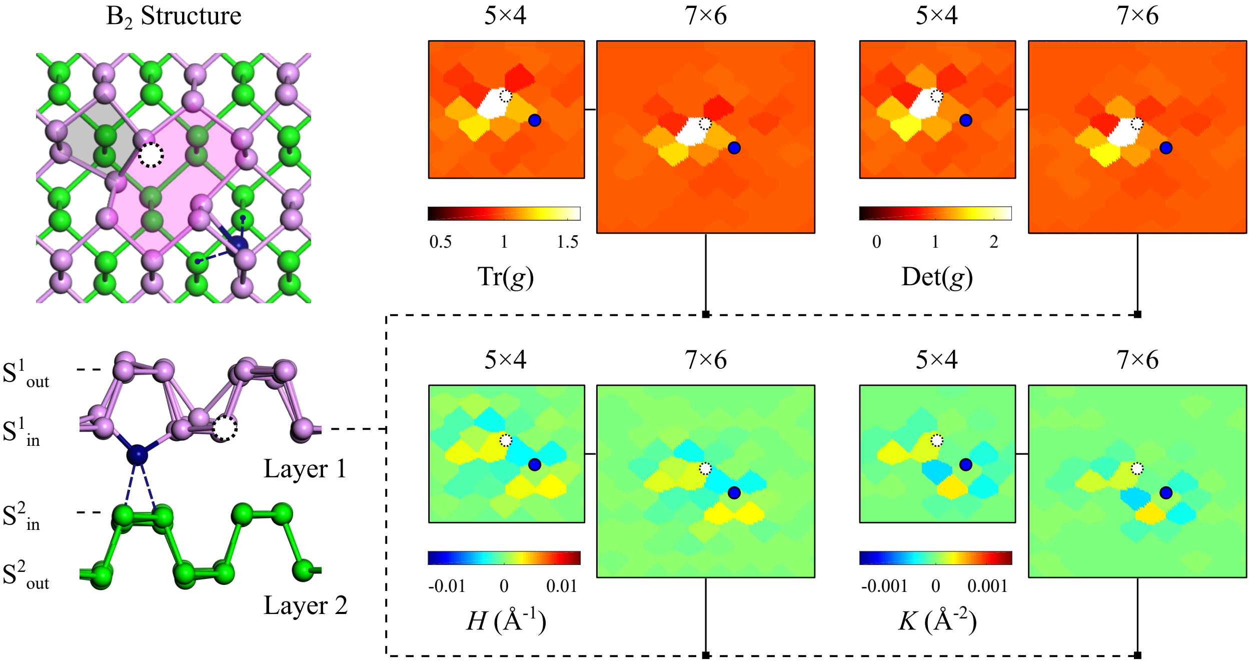


FIG. S3. Validation of the 5×4 supercell model. Discrete geometry results obtained for the 5×4 supercell are compared against those for a 7×6 supercell and verified to be independent of model size.

TABLE S1. The relaxed geometry, cohesive energy and UBER-fitted parameters (before and after DFT optimization) of AA-,AB-, AC- and AD-stacked bilayer phosphorene. Relevant data obtained for the monolayer are also included to provide a basis for comparison.

| | | Monolayer | Bilayer | | | |
|---|---|---|---|---|---|---|
| | | | AA | AB | AC | AD |
| Lattice constants | $a$ (Å) | 3.313 | 3.320 | 3.325 | 3.323 | 3.327 |
| | $b$ (Å) | 4.576 | 4.545 | 4.549 | 4.573 | 4.565 |
| Bond lengths | $r_1$ (Å) | 2.233 | 2.240 | 2.241 | 2.239 | 2.242 |
| | $r_1$' (Å) | 2.233 | 2.233 | 2.236 | 2.236 | 2.237 |
| | $r_2$ (Å) | 2.276 | 2.282 | 2.278 | 2.276 | 2.275 |
| Bond angles | $\theta_1$ (°) | 95.80 | 95.62 | 95.76 | 95.78 | 95.79 |
| | $\theta_1$' (°) | 95.80 | 96.00 | 96.05 | 95.95 | 96.07 |
| | $\theta_2$ (°) | 103.48 | 103.15 | 103.19 | 103.41 | 103.34 |
| | $\theta_2$' (°) | 103.48 | 103.10 | 103.15 | 103.39 | 103.31 |
| Thickness | $t$ (Å) | 2.134 | 2.147 | 2.142 | 2.136 | 2.136 |
| Cohesive energy | $E_c$ (eV/atom) | 3.462 | 3.507 | 3.517 | 3.499 | 3.508 |
| UBER-fitted (DFT-optimized) parameters | | $E_0$ (J/m$^2$) | -0.173 (-0.190) | -0.218 (-0.231) | -0.146 (-0.154) | -0.188 (-0.195) |
| | | $d_0$ (Å) | 3.599 (3.551) | 3.240 (3.197) | 3.805 (3.769) | 3.435 (3.399) |
| | | $E_b''(d_0)$ (GPa/Å) | 3.270 | 3.756 | 2.920 | 3.546 |

TABLE S2. The predicted band gap (in eV) of few-layer black phosphorus given by the Perdew-Burke-Ernzerhof (PBE),[7] optB88-vdW and hybrid Heyd-Scuseria-Ernzerhof (HSE06)[8,9] functionals, respectively.

| System | This work | | | Literature | |
|---|---|---|---|---|---|
| | PBE | optB88-vdW | HSE06 | HSE06 | Experimental |
| Monolayer | 0.814 | 0.825 | 1.488 | 1.52,[10] 1.51[11] | 1.45[12] |
| Bilayer | 0.438 | 0.460 | 1.054 | 1.04,[1] 1.02[10,11] | - |
| Bulk | ∼0 | ∼0 | 0.395 | 0.36,[1,11] 0.39[10] | 0.31 - 0.35[13–16] |
